# Supplementary material for: Adaptive Pre-training Data Detection for Large Language Models via Surprising Tokens
Source: arXiv:2407.21248 source file (2024-07-30)
Supplement: Supplementary file 1 [file appendix.tex]

% \section{Appendix / supplemental material}
\section{Implementation of \model}
In this section, we provide pseudocode for our proposed method \model, i.e, adaptively pre-training data detection via SURPrising tokens. 
\label{app:algo}
% Optionally include supplemental material (complete proofs, additional experiments and plots) in appendix.
% All such materials \textbf{SHOULD be included in the main submission.}

% \subsection{Algorithms}
% \label{app:algo}
\begin{algorithm}[h]
\small
\caption{SURP (pre-training data detection via surprising tokens)}
\begin{algorithmic}[1]
\State \textbf{Input:} A sequence of input tokens $x = x_1, x_2, ..., x_N$, Entropy threshold $\varepsilon_e$, probability parameter $k$, decision threshold $\lambda$
\State \textbf{Output:} Membership of the sequence $x$
% \State Initialize $S \gets \emptyset$
\For{$i=1$ to $N$}
\State Compute $P_{i,v_j} = p(v_j | x_1, \dots, x_{i-1}), \forall~v_j \in \mathcal{V}$, where $\mathcal{V}$ is the set of vocabulary
\State Compute entropy $E_i = -\sum_{v_j\in \mathcal{V}}P_{i,v_j}\log{P_{i,v_j}}$
\State Compute log probability $L_{i, v_j} = \log P_{i,v_j}$
\EndFor
\State $S_e=\{\}$
\For{$i=1$ to $N$}
    \If{$E_i < \varepsilon_e$}
        \State add $i$ to $S_e$
    \EndIf
\EndFor
% \State Select the tokens from $x$ with entropy smaller than $\varepsilon_e$, and add to set $S_e$. i.e., $S_e = \{i \mid \text{if } E_i < \varepsilon_e\}$
\State $L=[L_1, L_2, \dots, L_N]$
\State $L^k=percentile(L, k)$ \Comment{find $k$-th percentile of $L$}
\State $S_p=\{\}$
\For{$i=1$ to $N$}
    \If{$L_i < L^k$}
        \State add $i$ to $S_p$
    \EndIf
\EndFor
% \State Determine the $k$-th percentile $L^k$ of the set of log probabilities $\{L_1, L_2, \dots, L_N\}$. Then get set $S_p = \{i \mid \text{if } L_i < L^k\}$
\State $\model(x)= \frac{1}{\mid S_p\cap S_e \mid}\sum_{i \in S_p\cap S_e}{ L_{i, x_i}}$ 
% \State sort tokens from low to high with log probability $L_{i, x_i}$, and add token $x_i$ to set $S_p$ if $x_i\in S_e$, until $k$\% of $N$ tokens are added or all tokens are checked
% \State $\model(x)= \frac{1}{\mid S_p \mid}\sum_{x_i \in S_p}{ L_{i, x_i}}$ \Comment{double check whether - should be included}
% \State Select the top $k$\% of tokens from $x$ with the lowest probability and add to Min-k\%($x$)
% \State $\model(x)= \sum_{x_i \in \text{Min-k\%}(x)}{ -\log p(x_i | x_1, ..., x_{i-1})}$
\State \textbf{If} $\model(x) < \lambda$ \textbf{:} \textbf{return} Unseen \hspace{0.5cm} \textbf{Else:} \textbf{return} Seen
\end{algorithmic} \label{alg:1}
\end{algorithm}

\section{Compute Resources}
\label{app:compute}
Most of our experiments are done with GPUs. We use single GPU for each experiment running. 
We run experiments on NVIDIA RTX8000 with 48 GB memory limitation and NVIDIA V100 with 32 GB memory limitation. The exact experiment time varied depended on dataset, model, and method. 
% \clearpage

\section{Ethical Considerations}
\label{app:ethical}
This work conducts research on pre-training data detection problem, which aims to provide protection on the privacy data and copyrighted data under the current scenario of lacking transparency of training data in LLMs. 
Our method is for detection, so the text to detect comes from the user, and the text is required for our method. Wrongly use of our method will still be limited by the requirement. Therefore, our method cannot be used to extract information. This is the key difference of our method from the works about training data extraction, which could be misused to extract the privacy information. As a result, our method is defensive and will not do harm to privacy.
Our code will be released for research use. 
Regarding to the data we used, we do not see any issues. All existing data sets are publicly available and have been used for a long time in NLP research.
Our new data comes from \href{https://www.gutenberg.org/}{gutenberg.org}, which is an online library of over 70k ebooks. The books are older works for which U.S. copyright has expired. We don't see any issues in our dataset, as previously people use this source to construct data.
% diff from training data extraction, as we need a given text. so our method won't do harm to privacy, as extraction.
% Wrongly use of our method cannot extract information.
% Our code will be released for research use. 
% regard the data we use, we dont find any issue, as they are used for a long time
% our new data comes from which

\clearpage
\section{More Results}
\label{app:other_results}

\subsection{More Results on WikiMIA}
\label{app:wikimia}

\begin{table*}[th]
\caption{AUC-ROC scores for pre-training data detection on WikiMIA and various models across \model and baseline methods. Show results of the input length to be 64 and 256 respectively. \textbf{Bold} shows the best score of each column.}\label{tab:app_wikimia_results}
\begin{center} 
% \scriptsize
\setlength{\tabcolsep}{0.8pt}
\begin{tabularx}{\textwidth}{l *{14}{>{\centering\arraybackslash}X}@{}}
    \toprule
     \multirow{2}{*}{} & \multicolumn{2}{c}{LLaMA-7B} & \multicolumn{2}{c}{LLaMA-13B} & \multicolumn{2}{c}{Pythia-2.8B} & \multicolumn{2}{c}{Pythia-6.9B} & \multicolumn{2}{c}{Pythia-12B} & \multicolumn{2}{c}{GPT-neo-2.7B} \\
    \cmidrule(lr){2-3}  \cmidrule(lr){4-5} \cmidrule(lr){6-7} \cmidrule(lr){8-9} \cmidrule(lr){10-11} \cmidrule(lr){12-13}
    \textbf{Method} & 64 & 256
    & 64 & 256
    & 64 & 256
    & 64 & 256
    & 64 & 256
    & 64 & 256
    \\
    \midrule
        PPL & 0.614 & 0.696 & 0.636 & 0.713 & 0.584 & 0.678 & 0.607 & 0.686 & 0.619 & 0.695 & 0.585 & 0.669 \\
        Ref & 0.582 & 0.602 & 0.598 & 0.618 & 0.596 & 0.636 & 0.624 & 0.641 & 0.630 & 0.649 & 0.576 & 0.614 \\
        Lower & 0.586 & 0.656 & 0.620 & 0.656 & 0.578 & 0.629 & 0.582 & 0.595 & 0.596 & 0.632 & 0.577 & 0.641 \\
        Zlib & 0.634 & 0.712 & 0.653 & 0.732 & 0.606 & 0.693 & 0.626 & 0.698 & 0.635 & 0.708 & 0.607 & 0.681 \\
        Neighbor & 0.566 & 0.695 & 0.598 & 0.710 & 0.549 & 0.734 & 0.573 & 0.724 & 0.570 & 0.703 & 0.576 & 0.714 \\
        MinK & 0.634 & 0.703 & 0.660 & 0.727 & 0.612 & 0.700 & 0.650 & 0.717 & 0.665 & 0.736 & 0.628 & 0.694 \\
        \model & \textbf{0.842} & \textbf{0.786} & \textbf{0.856} & \textbf{0.801} & \textbf{0.622} & \textbf{0.734} & \textbf{0.658} & \textbf{0.725} & \textbf{0.683} & \textbf{0.743} & \textbf{0.635} & \textbf{0.719} \\
    \bottomrule
\end{tabularx}
\end{center}
% \vskip -0.1in
\end{table*}

\subsection{More Results on Dolma-Book}
\label{app:dolma}
\begin{table*}[th!]
\caption{AUC-ROC results for pre-training data detection on three datasets (\textit{head}, \textit{middle}, \textit{tail}) in Dolma-Book, using different sizes of OLMo models across \model and baseline methods. Each input text has the word length to be $512$.  \textbf{Bold} shows the best score of each column. Results show similar performance with $1024$ word-length inputs in \S \ref{subsec:eval_main}. }\label{tab:dolma512_results}
\begin{center} 
% \scriptsize
% \setlength{\tabcolsep}{0.8pt}
\begin{tabularx}{\textwidth}{l *{8}{>{\centering\arraybackslash}X}@{}}
    \toprule
     \multirow{2}{*}{} & \multicolumn{2}{c}{Dolma-Book-head-512} & \multicolumn{2}{c}{Dolma-Book-middle-512} & \multicolumn{2}{c}{Dolma-Book-tail-512}  \\
    \cmidrule(lr){2-3}  \cmidrule(lr){4-5} \cmidrule(lr){6-7}
    \textbf{Method} & OLMO-1B & OLMO-7B
    & OLMO-1B & OLMO-7B
    & OLMO-1B & OLMO-7B
    \\
    \midrule
        PPL & 0.610 & 0.583 & 0.610 & 0.604 & 0.575 & 0.569 \\
        Ref & - & 0.293 & - & 0.443 & - & 0.416 \\
        Lower & 0.428 & 0.426 & 0.522 & 0.505 & 0.459 & 0.451 \\
        Zlib & \textbf{0.753} & \textbf{0.752} & 0.459 & 0.460 & 0.543 & 0.540 \\
        % Neighbor &  \\
        MinK & 0.566 & 0.568 & 0.574 & 0.578 & 0.577 & 0.580 \\
        \model & 0.637 & 0.619 & \textbf{0.634} & \textbf{0.632} & \textbf{0.605} & \textbf{0.606} \\
    \bottomrule
\end{tabularx}
\end{center}
% \vskip -0.1in
\end{table*}

\subsection{Deduped Model Results.}
\label{app:deduped}
\begin{table*}[th!]
\caption{Compare the performance using Pythia-2.8B (Ori.) and deduped-Pythia-2.8B (De.) models. Show AUC-ROC results for pre-training data detection on seven datasets in MIMIR using SURP and baseline methods. Highlight best results as bold.}\label{tab:deduped_compare}
\begin{center} 
\scriptsize
\begin{tabularx}{\textwidth}{l *{18}{>{\centering\arraybackslash}X}@{}}
    \toprule
     \multirow{2}{*}{} & \multicolumn{2}{c}{Wikipedia} & \multicolumn{2}{c}{Github} & \multicolumn{2}{c}{Pile-CC} & \multicolumn{2}{c}{PubMed Central} & \multicolumn{2}{c}{Arxiv} & \multicolumn{2}{c}{DM Math} & \multicolumn{2}{c}{HackerNews} \\
    \cmidrule(lr){2-3}  \cmidrule(lr){4-5} \cmidrule(lr){6-7} \cmidrule(lr){8-9}  \cmidrule(lr){10-11} \cmidrule(lr){12-13} \cmidrule(lr){14-15} 
    \textbf{Method} & De. & Ori.
    & De. & Ori.
    & De. & Ori.
    & De. & Ori.
    & De. & Ori.
    & De. & Ori.
    & De. & Ori.
    \\
    \midrule
        PPL & 0.662 & 0.663 & 0.880 & 0.880 & 0.550 & 0.549 & 0.781 & 0.781 & 0.781 & 0.780 & 0.918 & 0.919 & 0.606 & 0.606 \\
        Ref & 0.560 & 0.561 & 0.417 & 0.418 & 0.530 & 0.530 & 0.391 & 0.392 & 0.565 & 0.565 & 0.380 & 0.377 & 0.520 & 0.522 \\
        Lower & 0.648 & 0.648 & 0.870 & 0.869 & 0.548 & 0.548 & 0.724 & 0.724 & 0.736 & 0.737 & 0.928 & 0.928 & 0.540 & 0.540 \\
        Zlib & 0.629 & 0.630 & \textbf{0.907} & \textbf{0.907} & 0.537 & 0.537 & 0.771 & 0.771 & 0.775 & 0.775 & 0.812 & 0.811 & 0.594 & 0.594 \\
        Neighbor & 0.571 & 0.572 & 0.868 & 0.868 & 0.482 & 0.480 & 0.618 & 0.617 & 0.659 & 0.664 & 0.746 & 0.752 & 0.534 & 0.538 \\
        MinK & 0.656 & 0.657 & 0.878 & 0.879 & 0.548 & 0.547 & 0.781 & 0.781 & 0.752 & 0.752 & 0.926 & 0.926 & 0.580 & 0.582 \\
        \model & \textbf{0.666} & \textbf{0.669} & 0.881 & 0.881 & \textbf{0.559} & \textbf{0.553} & \textbf{0.790} & \textbf{0.789} & \textbf{0.783} & \textbf{0.784} & \textbf{0.941} & \textbf{0.942} & \textbf{0.606} & \textbf{0.606} \\
    \bottomrule
\end{tabularx}
\end{center}
\end{table*}

\clearpage
\subsection{Results on Temporal Datasets.}
\label{app:temporal}
\begin{table*}[th!]
\caption{AUC-ROC results for pre-training data detection using Pythia-6.9B on temporal datasets (containing data distribution shifts) and common datasets (no data distribution shifts). Datasets are provided by \cite{duan2024membership}. The temporal datasets are created with training/non-training texts in different time periods. The common datasets of training/non-training texts are sampled from the train/test sets of the Pile dataset (i.e, which are within the same time range). 
}\label{tab:data_distribution_results}
\begin{center} 
% \scriptsize
% \setlength{\tabcolsep}{0.8pt}
\begin{tabularx}{\textwidth}{l *{5}{>{\centering\arraybackslash}X}@{}}
    \toprule
    \textbf{Method} & Wikipedia & Wiki-temporal & Arxiv & Arxiv-temporal \\
    \midrule
        PPL & 0.679 & 0.694 & 0.791 & 0.710 \\
        Ref & 0.582 & 0.568 & 0.586 & 0.624 \\
        Lower & 0.669 & 0.713 & 0.746 & 0.732 \\
        Zlib & 0.649 & 0.627 & 0.784 & 0.660 \\
        Neighbor & 0.567 & 0.606 & 0.670 & 0.633 \\
        MinK & 0.679 & 0.735 & 0.767 & 0.732 \\
        \model & \textbf{0.688} & \textbf{0.756} & \textbf{0.793} & \textbf{0.734} \\
    \bottomrule
\end{tabularx}
\end{center}
% \vskip -0.1in
\end{table*}

\subsection{Heatmap of AUC}
\label{app:heatmap}
\begin{figure}[th!]
    \centering
    \includegraphics[width=0.7\textwidth]{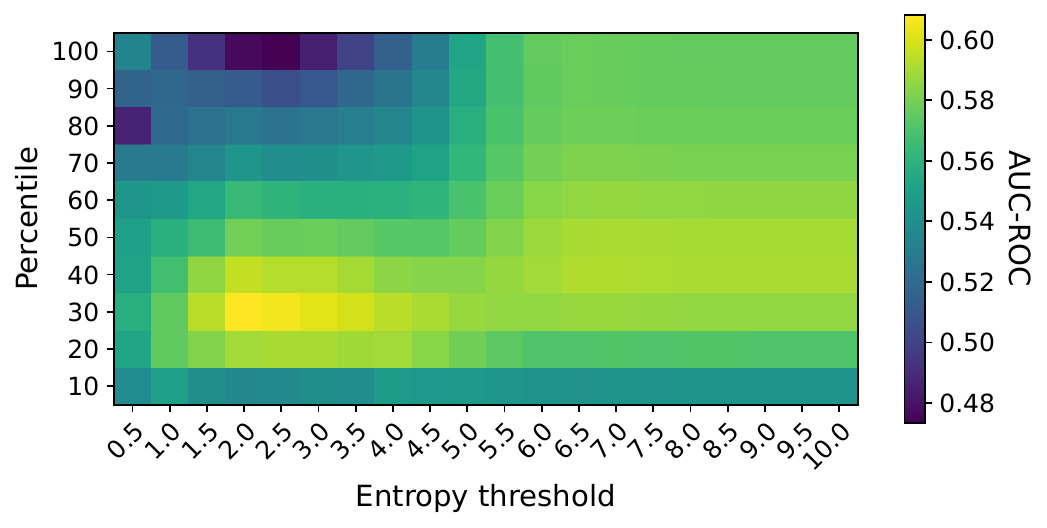}
    \caption{Another heatmap to show the AUC scores of different hyperparameters, using OLMo-7B on Dolma-Book-tail dataset.  The best AUC is achieved at low entropy ($\varepsilon_e=2.0$) and $k=30$.}
    \label{fig:other_heatmap}
\end{figure}

\section{TPR and FPR Tables}
\label{app:tpr_fpr}
\begin{table*}[h]
\caption{TPR@1\%FPR score for detecting the pre-trainig input examples from the given model on WikiMIA length-32/128 datasets for \model and baseline methods. }\label{tab:tpr_fpr1_wikimia}
\begin{center} 
% \scriptsize
\setlength{\tabcolsep}{0.8pt}
\begin{tabularx}{\textwidth}{l *{14}{>{\centering\arraybackslash}X}@{}}
    \toprule
     \multirow{2}{*}{} & \multicolumn{2}{c}{LLaMA-7B} & \multicolumn{2}{c}{LLaMA-13B} & \multicolumn{2}{c}{Pythia-2.8B} & \multicolumn{2}{c}{Pythia-6.9B} & \multicolumn{2}{c}{Pythia-12B} & \multicolumn{2}{c}{GPT-neo-2.7B} \\
    \cmidrule(lr){2-3}  \cmidrule(lr){4-5} \cmidrule(lr){6-7} \cmidrule(lr){8-9} \cmidrule(lr){10-11} \cmidrule(lr){12-13}
    \textbf{Method} & 32 & 128
    & 32 & 128
    & 32 & 128
    & 32 & 128
    & 32 & 128
    & 32 & 128
    \\
    \midrule
        PPL & 0.044 & 0.065 & 0.047 & 0.079 & 0.065 & 0.014 & 0.065 & 0.036 & 0.070 & 0.036 & 0.054 & 0.022 \\
        Ref & 0.021 & 0.058 & 0.023 & 0.065 & 0.016 & 0.007 & 0.018 & 0.014 & 0.028 & 0.007 & 0.026 & 0.000 \\
        Lower & 0.028 & 0.014 & 0.057 & 0.058 & 0.013 & 0.029 & 0.023 & 0.058 & 0.057 & 0.050 & 0.010 & 0.065 \\
        Zlib & 0.054 & 0.101 & 0.057 & 0.129 & 0.041 & 0.072 & 0.049 & 0.115 & 0.088 & 0.101 & 0.044 & 0.058 \\
        Neighbor & 0.010 & 0.040 & 0.005 & 0.020 & 0.000 & 0.050 & 0.000 & 0.070 & 0.000 & 0.010 & 0.000 & 0.060 \\
        MinK & 0.075 & 0.108 & 0.052 & 0.151 & 0.047 & 0.043 & 0.088 & 0.072 & 0.101 & 0.072 & 0.039 & 0.065 \\
        \model & 0.085 & 0.007 & 0.031 & 0.245 & 0.054 & 0.036 & 0.093 & 0.072 & 0.101 & 0.072 & 0.065 & 0.058 \\
    \bottomrule
\end{tabularx}
\end{center}
\end{table*}

\begin{table*}[h]
\caption{TPR@5\%FPR score for detecting the pre-trainig input examples from the given model on WikiMIA length-32/128 datasets for \model and baseline methods. }\label{tab:tpr_fpr5_wikimia}
\begin{center} 
% \scriptsize
\setlength{\tabcolsep}{0.8pt}
\begin{tabularx}{\textwidth}{l *{14}{>{\centering\arraybackslash}X}@{}}
    \toprule
     \multirow{2}{*}{} & \multicolumn{2}{c}{LLaMA-7B} & \multicolumn{2}{c}{LLaMA-13B} & \multicolumn{2}{c}{Pythia-2.8B} & \multicolumn{2}{c}{Pythia-6.9B} & \multicolumn{2}{c}{Pythia-12B} & \multicolumn{2}{c}{GPT-neo-2.7B} \\
    \cmidrule(lr){2-3}  \cmidrule(lr){4-5} \cmidrule(lr){6-7} \cmidrule(lr){8-9} \cmidrule(lr){10-11} \cmidrule(lr){12-13}
    \textbf{Method} & 32 & 128
    & 32 & 128
    & 32 & 128
    & 32 & 128
    & 32 & 128
    & 32 & 128
    \\
    \midrule
        PPL & 0.119 & 0.187 & 0.140 & 0.216 & 0.147 & 0.094 & 0.142 & 0.144 & 0.171 & 0.180 & 0.158 & 0.122 \\
        Ref & 0.059 & 0.072 & 0.062 & 0.079 & 0.062 & 0.101 & 0.067 & 0.137 & 0.090 & 0.122 & 0.072 & 0.072 \\
        Lower & 0.106 & 0.094 & 0.096 & 0.158 & 0.111 & 0.108 & 0.106 & 0.129 & 0.163 & 0.129 & 0.083 & 0.137 \\
        Zlib & 0.137 & 0.144 & 0.116 & 0.187 & 0.158 & 0.187 & 0.163 & 0.209 & 0.171 & 0.237 & 0.150 & 0.173 \\
        Neighbor & 0.085 & 0.200 & 0.070 & 0.110 & 0.075 & 0.190 & 0.085 & 0.160 & 0.080 & 0.090 & 0.065 & 0.180 \\
        MinK & 0.152 & 0.194 & 0.189 & 0.201 & 0.165 & 0.137 & 0.178 & 0.180 & 0.230 & 0.201 & 0.217 & 0.144 \\
        \model & 0.279 & 0.410 & 0.287 & 0.475 & 0.168 & 0.108 & 0.233 & 0.180 & 0.251 & 0.223 & 0.209 & 0.230 \\
    \bottomrule
\end{tabularx}
\end{center}
\end{table*}

\begin{table*}[h]
\caption{TPR@10\%FPR score for detecting the pre-trainig input examples from the given model on WikiMIA length-32/128 datasets for \model and baseline methods.}\label{tab:tpr_fpr10_wikimia}
\begin{center} 
% \scriptsize
\setlength{\tabcolsep}{0.8pt}
\begin{tabularx}{\textwidth}{l *{14}{>{\centering\arraybackslash}X}@{}}
    \toprule
     \multirow{2}{*}{} & \multicolumn{2}{c}{LLaMA-7B} & \multicolumn{2}{c}{LLaMA-13B} & \multicolumn{2}{c}{Pythia-2.8B} & \multicolumn{2}{c}{Pythia-6.9B} & \multicolumn{2}{c}{Pythia-12B} & \multicolumn{2}{c}{GPT-neo-2.7B} \\
    \cmidrule(lr){2-3}  \cmidrule(lr){4-5} \cmidrule(lr){6-7} \cmidrule(lr){8-9} \cmidrule(lr){10-11} \cmidrule(lr){12-13}
    \textbf{Method} & 32 & 128
    & 32 & 128
    & 32 & 128
    & 32 & 128
    & 32 & 128
    & 32 & 128
    \\
    \midrule
        PPL & 0.209 & 0.273 & 0.292 & 0.309 & 0.233 & 0.252 & 0.222 & 0.259 & 0.222 & 0.266 & 0.212 & 0.194 \\
        Ref & 0.114 & 0.086 & 0.106 & 0.101 & 0.176 & 0.216 & 0.199 & 0.237 & 0.207 & 0.194 & 0.111 & 0.187 \\
        Lower & 0.176 & 0.187 & 0.214 & 0.180 & 0.196 & 0.165 & 0.214 & 0.194 & 0.274 & 0.223 & 0.168 & 0.201 \\
        Zlib & 0.204 & 0.259 & 0.245 & 0.273 & 0.225 & 0.216 & 0.220 & 0.281 & 0.248 & 0.295 & 0.209 & 0.302 \\
        Neighbor & 0.165 & 0.220 & 0.135 & 0.140 & 0.140 & 0.310 & 0.170 & 0.270 & 0.250 & 0.200 & 0.150 & 0.240 \\
        MinK & 0.207 & 0.338 & 0.258 & 0.338 & 0.225 & 0.230 & 0.284 & 0.374 & 0.315 & 0.295 & 0.271 & 0.230 \\
        \model & 0.571 & 0.561 & 0.641 & 0.583 & 0.251 & 0.237 & 0.313 & 0.353 & 0.331 & 0.317 & 0.297 & 0.288 \\
    \bottomrule
\end{tabularx}
\end{center}
\end{table*}

\begin{table*}[h]
\caption{TPR@1\%FPR score for detecting the pre-trainig input examples from the given model on WikiMIA length-64/256 datasets for \model and baseline methods.}\label{tab:tpr_fpr1_wikimia64}
\begin{center} 
% \scriptsize
\setlength{\tabcolsep}{0.8pt}
\begin{tabularx}{\textwidth}{l *{14}{>{\centering\arraybackslash}X}@{}}
    \toprule
     \multirow{2}{*}{} & \multicolumn{2}{c}{LLaMA-7B} & \multicolumn{2}{c}{LLaMA-13B} & \multicolumn{2}{c}{Pythia-2.8B} & \multicolumn{2}{c}{Pythia-6.9B} & \multicolumn{2}{c}{Pythia-12B} & \multicolumn{2}{c}{GPT-neo-2.7B} \\
    \cmidrule(lr){2-3}  \cmidrule(lr){4-5} \cmidrule(lr){6-7} \cmidrule(lr){8-9} \cmidrule(lr){10-11} \cmidrule(lr){12-13}
    \textbf{Method} & 64 & 256
    & 64 & 256
    & 64 & 256
    & 64 & 256
    & 64 & 256
    & 64 & 256
    \\
    \midrule
        PPL & 0.039 & 0.118 & 0.042 & 0.137 & 0.028 & 0.039 & 0.028 & 0.020 & 0.028 & 0.020 & 0.032 & 0.020 \\
        Ref & 0.018 & 0.020 & 0.021 & 0.039 & 0.028 & 0.039 & 0.032 & 0.020 & 0.014 & 0.020 & 0.025 & 0.000 \\
        Lower & 0.021 & 0.039 & 0.053 & 0.059 & 0.025 & 0.020 & 0.028 & 0.020 & 0.042 & 0.020 & 0.014 & 0.000 \\
        Zlib & 0.067 & 0.196 & 0.081 & 0.196 & 0.049 & 0.059 & 0.060 & 0.020 & 0.049 & 0.078 & 0.049 & 0.020 \\
        Neighbor & 0.020 & 0.097 & 0.055 & 0.097 & 0.005 & 0.032 & 0.000 & 0.065 & 0.035 & 0.032 & 0.010 & 0.161 \\
        MinK & 0.049 & 0.098 & 0.060 & 0.157 & 0.025 & 0.039 & 0.039 & 0.059 & 0.046 & 0.098 & 0.056 & 0.059 \\
        \model & 0.085 & 0.255 & 0.099 & 0.412 & 0.000 & 0.039 & 0.067 & 0.059 & 0.063 & 0.118 & 0.032 & 0.059 \\
    \bottomrule
\end{tabularx}
\end{center}
% \vskip -0.1in
\end{table*}

\begin{table*}[h]
\caption{TPR@5\%FPR score for detecting the pre-trainig input examples from the given model on WikiMIA length-64/256 datasets for \model and baseline methods.}\label{tab:tpr_fpr5_wikimia64}
\begin{center} 
% \scriptsize
\setlength{\tabcolsep}{0.8pt}
\begin{tabularx}{\textwidth}{l *{14}{>{\centering\arraybackslash}X}@{}}
    \toprule
     \multirow{2}{*}{} & \multicolumn{2}{c}{LLaMA-7B} & \multicolumn{2}{c}{LLaMA-13B} & \multicolumn{2}{c}{Pythia-2.8B} & \multicolumn{2}{c}{Pythia-6.9B} & \multicolumn{2}{c}{Pythia-12B} & \multicolumn{2}{c}{GPT-neo-2.7B} \\
    \cmidrule(lr){2-3}  \cmidrule(lr){4-5} \cmidrule(lr){6-7} \cmidrule(lr){8-9} \cmidrule(lr){10-11} \cmidrule(lr){12-13}
    \textbf{Method} & 64 & 256
    & 64 & 256
    & 64 & 256
    & 64 & 256
    & 64 & 256
    & 64 & 256
    \\
    \midrule
        PPL & 0.074 & 0.137 & 0.113 & 0.157 & 0.102 & 0.039 & 0.134 & 0.059 & 0.092 & 0.118 & 0.120 & 0.039 \\
        Ref & 0.088 & 0.039 & 0.088 & 0.059 & 0.106 & 0.039 & 0.120 & 0.059 & 0.130 & 0.059 & 0.081 & 0.078 \\
        Lower & 0.113 & 0.098 & 0.116 & 0.137 & 0.102 & 0.020 & 0.116 & 0.039 & 0.123 & 0.078 & 0.099 & 0.020 \\
        Zlib & 0.109 & 0.216 & 0.127 & 0.275 & 0.144 & 0.196 & 0.162 & 0.275 & 0.113 & 0.255 & 0.151 & 0.137 \\
        Neighbor & 0.075 & 0.129 & 0.100 & 0.226 & 0.065 & 0.226 & 0.065 & 0.129 & 0.080 & 0.258 & 0.040 & 0.194 \\
        MinK & 0.148 & 0.118 & 0.173 & 0.157 & 0.183 & 0.078 & 0.190 & 0.137 & 0.215 & 0.137 & 0.183 & 0.098 \\
        \model & 0.345 & 0.373 & 0.394 & 0.431 & 0.000 & 0.078 & 0.180 & 0.098 & 0.215 & 0.137 & 0.173 & 0.098 \\
    \bottomrule
\end{tabularx}
\end{center}
% \vskip -0.1in
\end{table*}

\begin{table*}[h]
\caption{TPR@10\%FPR score for detecting the pre-trainig input examples from the given model on WikiMIA length-64/256 datasets for \model and baseline methods.}\label{tab:tpr_fpr10_wikimia64}
\begin{center} 
% \scriptsize
\setlength{\tabcolsep}{0.8pt}
\begin{tabularx}{\textwidth}{l *{14}{>{\centering\arraybackslash}X}@{}}
    \toprule
     \multirow{2}{*}{} & \multicolumn{2}{c}{LLaMA-7B} & \multicolumn{2}{c}{LLaMA-13B} & \multicolumn{2}{c}{Pythia-2.8B} & \multicolumn{2}{c}{Pythia-6.9B} & \multicolumn{2}{c}{Pythia-12B} & \multicolumn{2}{c}{GPT-neo-2.7B} \\
    \cmidrule(lr){2-3}  \cmidrule(lr){4-5} \cmidrule(lr){6-7} \cmidrule(lr){8-9} \cmidrule(lr){10-11} \cmidrule(lr){12-13}
    \textbf{Method} & 64 & 256
    & 64 & 256
    & 64 & 256
    & 64 & 256
    & 64 & 256
    & 64 & 256
    \\
    \midrule
        PPL & 0.158 & 0.157 & 0.201 & 0.216 & 0.211 & 0.196 & 0.225 & 0.333 & 0.243 & 0.235 & 0.208 & 0.255 \\
        Ref & 0.134 & 0.118 & 0.141 & 0.098 & 0.187 & 0.118 & 0.208 & 0.098 & 0.225 & 0.078 & 0.151 & 0.078 \\
        Lower & 0.137 & 0.176 & 0.222 & 0.216 & 0.173 & 0.294 & 0.141 & 0.216 & 0.169 & 0.157 & 0.162 & 0.118 \\
        Zlib & 0.194 & 0.235 & 0.204 & 0.275 & 0.225 & 0.333 & 0.229 & 0.373 & 0.243 & 0.314 & 0.208 & 0.353 \\
        Neighbor & 0.105 & 0.258 & 0.150 & 0.323 & 0.115 & 0.290 & 0.105 & 0.355 & 0.190 & 0.323 & 0.100 & 0.387 \\
        MinK & 0.229 & 0.353 & 0.250 & 0.373 & 0.261 & 0.137 & 0.306 & 0.314 & 0.317 & 0.392 & 0.271 & 0.235 \\
        \model & 0.616 & 0.392 & 0.609 & 0.490 & 0.183 & 0.216 & 0.327 & 0.314 & 0.324 & 0.451 & 0.268 & 0.392 \\
    \bottomrule
\end{tabularx}
\end{center}
% \vskip -0.1in
\end{table*}

\begin{table*}[h]
\caption{TPR@5\%FPR score for detecting the pre-trainig input examples from the given model on three datasets(\textit{head}, \textit{middle}, \textit{tail}) in Dolma-Book for \model and baseline methods.}\label{tab:tpr_fpr5_dolma}
\begin{center} 
% \scriptsize
\setlength{\tabcolsep}{0.8pt}
\begin{tabularx}{\textwidth}{l *{8}{>{\centering\arraybackslash}X}@{}}
    \toprule
     \multirow{2}{*}{} & \multicolumn{2}{c}{Dolma-Book-head} & \multicolumn{2}{c}{Dolma-Book-middle} & \multicolumn{2}{c}{Dolma-Book-tail}  \\
    \cmidrule(lr){2-3}  \cmidrule(lr){4-5} \cmidrule(lr){6-7}
    \textbf{Method} & OLMO-1B & OLMO-7B
    & OLMO-1B & OLMO-7B
    & OLMO-1B & OLMO-7B
    \\
    \midrule
        PPL & 0.101 & 0.108 & 0.115 & 0.126 & 0.072 & 0.090 \\
        Ref & 0.000 & 0.048 & 0.000 & 0.033 & 0.000 & 0.027 \\
        Lower & 0.044 & 0.053 & 0.062 & 0.090 & 0.060 & 0.072 \\
        Zlib & 0.200 & 0.215 & 0.069 & 0.078 & 0.070 & 0.077 \\
        % Neighbor & - & 0.095 & 0.140 & - & - & - \\
        MinK & 0.065 & 0.086 & 0.106 & 0.121 & 0.078 & 0.097 \\
        \model & 0.098 & 0.116 & 0.122 & 0.134 & 0.088 & 0.112 \\
    \bottomrule
\end{tabularx}
\end{center}
\end{table*}

\begin{table*}[h]
\caption{TPR@5\%FPR score for detecting the pre-trainig input examples from the given model on seven datasets in MIMIR for \model and baseline methods.}\label{tab:tpr_fpr5_mimir}
\begin{center} 
\scriptsize
\setlength{\tabcolsep}{0.7pt}
\begin{tabularx}{\textwidth}{l *{18}{>{\centering\arraybackslash}X}@{}}
    \toprule
    \multirow{2}{*}{}  & \multicolumn{4}{c}{Wikipedia} & \multicolumn{4}{c}{Github} & \multicolumn{4}{c}{Pile CC} & \multicolumn{4}{c}{PubMed Central} \\
    \cmidrule(lr){2-5}  \cmidrule(lr){6-9} \cmidrule(lr){10-13} \cmidrule(lr){14-17}
    \textbf{Method} & Pythia-2.8B & Pythia-6.9B & Pythia-12B & Neo-2.7B
    & Pythia-2.8B & Pythia-6.9B & Pythia-12B & Neo-2.7B
    & Pythia-2.8B & Pythia-6.9B & Pythia-12B & Neo-2.7B
    & Pythia-2.8B & Pythia-6.9B & Pythia-12B & Neo-2.7B
    \\
    \midrule
        PPL & 0.228 & 0.240 & 0.242 & 0.233 & 0.571 & 0.619 & 0.631 & 0.552 & 0.112 & 0.137 & 0.139 & 0.125 & 0.320 & 0.305 & 0.314 & 0.348 \\
        Ref & 0.037 & 0.041 & 0.040 & 0.042 & 0.015 & 0.019 & 0.007 & 0.037 & 0.040 & 0.049 & 0.052 & 0.031 & 0.004 & 0.006 & 0.006 & 0.006 \\
        Lower & 0.137 & 0.144 & 0.140 & 0.118 & 0.545 & 0.571 & 0.578 & 0.575 & 0.051 & 0.050 & 0.057 & 0.040 & 0.049 & 0.051 & 0.053 & 0.022 \\
        Zlib & 0.091 & 0.101 & 0.107 & 0.092 & 0.481 & 0.496 & 0.511 & 0.526 & 0.054 & 0.066 & 0.076 & 0.052 & 0.145 & 0.124 & 0.100 & 0.181 \\
        Neighbor & 0.050 & 0.050 & 0.025 & 0.045 & 0.240 & 0.245 & 0.305 & 0.270 & 0.005 & 0.030 & 0.010 & 0.025 & 0.055 & 0.030 & 0.030 & 0.025 \\
        MinK & 0.120 & 0.141 & 0.127 & 0.086 & 0.470 & 0.500 & 0.515 & 0.463 & 0.049 & 0.053 & 0.054 & 0.044 & 0.191 & 0.212 & 0.224 & 0.236 \\
        \model & 0.236 & 0.248 & 0.259 & 0.235 & 0.571 & 0.612 & 0.634 & 0.552 & 0.083 & 0.135 & 0.143 & 0.125 & 0.358 & 0.346 & 0.338 & 0.365 \\
        \vspace{-.6em} \\
    \toprule
    \multirow{2}{*}{}  & & \multicolumn{4}{c}{ArXiv} & & \multicolumn{4}{c}{DM Math} & & \multicolumn{4}{c}{HackerNews} &  \\
    \cmidrule(lr){3-6}  \cmidrule(lr){8-11} \cmidrule(lr){13-16}
    \textbf{Method} &  & Pythia-2.8B & Pythia-6.9B & Pythia-12B & Neo-2.7B
     & & Pythia-2.8B & Pythia-6.9B & Pythia-12B & Neo-2.7B
     & & Pythia-2.8B & Pythia-6.9B & Pythia-12B & Neo-2.7B & 
    \\
    \midrule
        PPL         &  & 0.342 & 0.370 & 0.360 & 0.364 &  & 0.596 & 0.629 & 0.629 & 0.674 &  & 0.116 & 0.122 & 0.144 & 0.102 \\
        Ref         &  & 0.104 & 0.110 & 0.116 & 0.086 &  & 0.067 & 0.067 & 0.067 & 0.011 &  & 0.060 & 0.073 & 0.077 & 0.059 \\
        Lower       &  & 0.238 & 0.276 & 0.264 & 0.310 &  & 0.663 & 0.674 & 0.663 & 0.674 &  & 0.074 & 0.080 & 0.077 & 0.062 \\
        Zlib        &  & 0.320 & 0.330 & 0.332 & 0.328 &  & 0.169 & 0.169 & 0.169 & 0.236 &  & 0.105 & 0.118 & 0.133 & 0.098 \\
        Neighbor    &  & 0.170 & 0.135 & 0.190 & 0.125 &  & 0.140 & 0.300 & 0.400 & 0.360 &  & 0.075 & 0.100 & 0.075 & 0.080 \\
        MinK        &  & 0.348 & 0.352 & 0.368 & 0.360 &  & 0.697 & 0.697 & 0.708 & 0.730 &  & 0.110 & 0.105 & 0.122 & 0.087 \\
        \model      &  & 0.348 & 0.366 & 0.364 & 0.366 &  & 0.753 & 0.775 & 0.764 & 0.809 &  & 0.118 & 0.128 & 0.132 & 0.102 \\
    \bottomrule
\end{tabularx}
\end{center}
% \vskip -0.1in
\end{table*}
